# Supplementary material for: Reviving, reproducing, and revisiting Axelrod's second tournament
Source: arXiv:2510.15438 source file (2025-10-17)
Supplement: Supplementary file 1 [file si_list_of_all_strategies.tex]

\item EvolvedLookerUp2_2_2: 1 / 30 / 118
\item Evolved HMM 5: 2 / 13 / 59
\item Omega TFT: 3, 8: 3 / 4 / 17
\item Evolved ANN 5: 4 / 7 / 36
\item Evolved ANN: 5 / 3 / 8
\item Evolved FSM 16: 6 / 15 / 78
\item Evolved FSM 16 Noise 05: 7 / 1 / 4
\item PSO Gambler 2_2_2: 8 / 53 / 138
\item Original Gradual: 9 / 20 / 30
\item PSO Gambler 2_2_2 Noise 05: 10 / 9 / 24
\item PSO Gambler Mem1: 11 / 39 / 107
\item Evolved FSM 4: 12 / 28 / 85
\item PSO Gambler 1_1_1: 13 / 61 / 140
\item Gradual: 14 / 17 / 29
\item DBS: 0.75, 3, 4, 3, 5: 15 / 2 / 1
\item k42r: 16 / 25 / 21 / 3
\item Winner12: 17 / 60 / 127
\item Spiteful Tit For Tat: 18 / 24 / 22
\item k60r: 19 / 31 / 25 / 6
\item k85r: 20 / 57 / 101 / 33
\item EugineNier: (D,): 21 / 35 / 27
\item k80r: 22 / 10 / 3 / 36
\item k32r: 23 / 40 / 34 / 10
\item DoubleCrosser: (D, D): 24 / 11 / 13
\item k58r: 25 / 38 / 43 / 21
\item k87r: 26 / 74 / 124 / 44
\item k40r: 27 / 34 / 80 / 35
\item k65r: 28 / 5 / 18 / 47
\item Forgetful Fool Me Once: 0.05: 29 / 19 / 41
\item k49r: 30 / 32 / 23 / 4
\item k56r: 31 / 21 / 12 / 38
\item k59r: 32 / 23 / 11 / 40
\item Revised Downing: 33 / 22 / 10
\item Fool Me Once: 34 / 14 / 37
\item k41r: 35 / 33 / 40 / 7
\item k55r: 36 / 27 / 15 / 42
\item First by Shubik: 37 / 87 / 95
\item ZD-GTFT-2: 0.25, 0.5: 38 / 48 / 63
\item Soft Joss: 0.9: 39 / 49 / 56
\item BackStabber: (D, D): 40 / 8 / 9
\item MEM2: 41 / 79 / 103
\item AON2: 42 / 116 / 168
\item k81r: 43 / 6 / 14 / 43
\item Meta Hunter: 6 players: 44 / 69 / 108
\item NMWE Finite Memory: 79 players: 45 / 91 / 126
\item k44r: 46 / 37 / 26 / 5
\item k84r: 47 / 43 / 76 / 9
\item GTFT: 0.33: 48 / 55 / 72
\item EvolvedLookerUp1_1_1: 49 / 115 / 147
\item NMWE Stochastic: 67 players: 50 / 97 / 123
\item k38r: 51 / 26 / 7 / 34
\item Michaelos: (D,): 52 / 86 / 97
\item First by Stein and Rapoport: 0.05: (D, D): 53 / 47 / 44
\item NMWE Memory One: 36 players: 54 / 90 / 104
\item Resurrection: 55 / 65 / 67
\item Nice Meta Winner Ensemble: 213 players: 56 / 98 / 111
\item k92r: 57 / 70 / 69 / 1
\item Adaptive Tit For Tat: 0.5: 58 / 72 / 68
\item Forgiving Tit For Tat: 59 / 46 / 58
\item NMWE Deterministic: 146 players: 60 / 93 / 109
\item General Soft Grudger: n=1,d=4,c=2: 61 / 110 / 144
\item Soft Grudger: 62 / 109 / 142
\item Meta Majority Long Memory: 134 players: 63 / 62 / 62
\item Firm But Fair: 64 / 100 / 91
\item Level Punisher: 65 / 29 / 16
\item k68r: 66 / 117 / 139 / 12
\item k86r: 67 / 36 / 49 / 28
\item NMWE Long Memory: 134 players: 68 / 105 / 112
\item Meta Majority: 213 players: 69 / 66 / 75
\item ZD-GEN-2: 0.125, 0.5, 3: 70 / 99 / 110
\item k66r: 71 / 41 / 19 / 20
\item Evolved ANN 5 Noise 05: 72 / 12 / 2
\item Second by Eatherley: 73 / 64 / 79
\item k46r: 74 / 63 / 77 / 14
\item TF3: 75 / 75 / 90
\item Memory Decay: 0.1, 0.03, -2, 1, Tit For Tat, 15: 76 / 51 / 51
\item Nice Meta Winner: 213 players: 77 / 114 / 129
\item k72r: 78 / 77 / 38 / 13
\item k43r: 79 / 18 / 6 / 39
\item Doubler: 80 / 54 / 42
\item Meta Majority Finite Memory: 79 players: 81 / 59 / 64
\item GrudgerAlternator: 82 / 124 / 159
\item k34r: 83 / 111 / 119 / 52
\item k47r: 84 / 16 / 5 / 16
\item k61r: 85 / 126 / 156 / 2
\item Second by Champion: 86 / 108 / 93
\item k35r: 87 / 95 / 89 / 11
\item k79r: 88 / 52 / 54 / 26
\item k91r: 89 / 67 / 52 / 30
\item ShortMem: 90 / 56 / 32
\item Dynamic Two Tits For Tat: 91 / 94 / 92
\item k64r: 92 / 71 / 46 / 17
\item Adaptive Pavlov 2011: 93 / 112 / 121
\item First by Tideman and Chieruzzi: (D, D): 94 / 120 / 102
\item Adaptive Pavlov 2006: 95 / 113 / 131
\item Meta Majority Memory One: 36 players: 96 / 101 / 87
\item Once Bitten: 97 / 45 / 39
\item First by Davis: 10: 98 / 127 / 122
\item k53r: 99 / 128 / 128 / 45
\item Soft Go By Majority: 5: 100 / 50 / 35
\item k73r: 101 / 44 / 50 / 41
\item Limited Retaliate 3: 0.05, 20: 102 / 130 / 152
\item Inverse Punisher: 103 / 132 / 157
\item k70r: 104 / 129 / 149 / 32
\item Forgiver: 105 / 82 / 96
\item k83r: 106 / 92 / 83 / 15
\item Limited Retaliate 2: 0.08, 15: 107 / 134 / 164
\item Slow Tit For Two Tats 2: 108 / 68 / 74
\item First by Grofman: 109 / 135 / 176
\item k75r: 110 / 42 / 31 / 8
\item Stalker: (D,): 111 / 88 / 65
\item VeryBad: 112 / 89 / 60
\item k37r: 113 / 73 / 57 / 37
\item Hard Tit For 2 Tats: 114 / 83 / 70
\item k57r: 115 / 147 / 182 / 31
\item Soft Go By Majority: 10: 116 / 76 / 47
\item Soft Go By Majority: 20: 117 / 84 / 55
\item Soft Go By Majority: 40: 118 / 96 / 66
\item Limited Retaliate: 0.1, 20: 119 / 138 / 170
\item Nice Average Copier: 120 / 123 / 133
\item Worse and Worse 3: 121 / 125 / 132
\item Punisher: 122 / 137 / 167
\item Retaliate 2: 0.08: 123 / 139 / 163
\item Second by Appold: 124 / 119 / 106
\item Retaliate 3: 0.05: 125 / 133 / 153
\item k88r: 126 / 122 / 113 / 22
\item k31r: 127 / 107 / 73 / 23
\item Math Constant Hunter: 128 / 136 / 146
\item Forgetful Grudger: 129 / 144 / 172
\item k39r: 130 / 81 / 20 / 25
\item Retaliate: 0.1: 131 / 143 / 171
\item k90r: 132 / 104 / 71 / 24
\item Grumpy: Nice, 10, -10: 133 / 118 / 88
\item N Tit(s) For M Tat(s): 3, 2: 134 / 85 / 81
\item Thumper: 135 / 148 / 161
\item Two Tits For Tat: 136 / 146 / 165
\item Inverse: 137 / 140 / 148
\item Delayed AON1: 138 / 152 / 215
\item Hard Tit For Tat: 139 / 150 / 178
\item Tricky Level Punisher: 140 / 106 / 117
\item Appeaser: 141 / 155 / 205
\item Win-Stay Lose-Shift: 142 / 156 / 206
\item AdaptorBrief: 143 / 78 / 53
\item k69r: 144 / 121 / 48 / 29
\item k78r: 145 / 80 / 61 / 19
\item k67r: 146 / 103 / 33 / 27
\item Eventual Cycle Hunter: 147 / 157 / 198
\item k82r: 148 / 58 / 28 / 49
\item First by Nydegger: 149 / 153 / 173
\item First by Graaskamp: 0.05: 150 / 102 / 82
\item k48r: 151 / 141 / 94 / 53
\item Random Hunter: 152 / 154 / 154
\item UsuallyCooperates: 153 / 183 / 230
\item Cycle Hunter: 154 / 169 / 193
\item k76r: 155 / 166 / 155 / 46
\item Second by Tester: 156 / 163 / 151
\item Defector Hunter: 157 / 173 / 204
\item Raider: 158 / 161 / 134
\item Alternator Hunter: 159 / 175 / 200
\item AdaptorLong: 160 / 149 / 169
\item Ripoff: 161 / 172 / 162
\item Average Copier: 162 / 171 / 177
\item k45r: 163 / 159 / 115 / 50
\item k51r: 164 / 167 / 158 / 18
\item Prober 2: 165 / 162 / 130
\item k33r: 166 / 178 / 145 / 59
\item Knowledgeable Worse and Worse: 167 / 181 / 214
\item Cooperator: 168 / 179 / 211
\item k52r: 169 / 151 / 100 / 48
\item k77r: 170 / 131 / 45 / 55
\item Hard Prober: 171 / 164 / 125
\item Sneaky Tit For Tat: 172 / 180 / 179
\item k62r: 173 / 158 / 99 / 51
\item DoubleResurrection: 174 / 165 / 105
\item k89r: 175 / 200 / 191 / 56
\item Suspicious Tit For Tat: 176 / 185 / 160
\item Willing: 177 / 192 / 203
\item Remorseful Prober: 0.1: 178 / 168 / 114
\item First by Feld: 1.0, 0.5, 200: 179 / 145 / 84
\item First by Downing: 180 / 174 / 86
\item ZD-Mem2: 181 / 170 / 141
\item Worse and Worse 2: 182 / 142 / 98
\item Risky QLearner: 183 / 195 / 217
\item Cautious QLearner: 184 / 194 / 218
\item Arrogant QLearner: 185 / 196 / 216
\item Hesitant QLearner: 186 / 197 / 219
\item Detective: 187 / 189 / 166
\item Random Tit for Tat: 0.5: 188 / 188 / 180
\item First by Tullock: 189 / 160 / 116
\item k74r: 190 / 186 / 120 / 61
\item k54r: 191 / 191 / 143 / 58
\item Adaptive: 192 / 184 / 150
\item Worse and Worse: 193 / 190 / 212
\item Prober: 194 / 193 / 174
\item Hard Go By Majority: 5: 195 / 198 / 181
\item Hard Go By Majority: 196 / 202 / 194
\item Opposite Grudger: 197 / 208 / 236
\item Stochastic Cooperator: 198 / 187 / 187
\item Pun1: 199 / 206 / 199
\item Naive Prober: 0.1: 200 / 177 / 137
\item EasyGo: 201 / 220 / 259
\item First by Joss: 0.9: 202 / 176 / 136
\item ALLCorALLD: 203 / 211 / 228
\item Hard Go By Majority: 40: 204 / 201 / 188
\item Prober 4: 205 / 203 / 183
\item Prober 3: 206 / 199 / 175
\item Hard Go By Majority: 20: 207 / 207 / 185
\item Calculator: 208 / 182 / 135
\item Hard Go By Majority: 10: 209 / 209 / 186
\item SolutionB5: 210 / 210 / 184
\item Winner21: 211 / 221 / 225
\item Meta Mixer: 213 players: 212 / 205 / 195
\item Fortress3: 213 / 223 / 226
\item Fortress4: 214 / 224 / 222
\item Meta Hunter Aggressive: 7 players: 215 / 212 / 202
\item Cycler CCCCCD: 216 / 219 / 238
\item Stochastic WSLS: 0.05: 217 / 204 / 229
\item Cycler CCCDCD: 218 / 227 / 244
\item k71r: 219 / 222 / 220 / 60
\item Cycler CCCD: 220 / 228 / 245
\item ZD-SET-2: 0.25, 0.0, 2: 221 / 215 / 210
\item TF2: 222 / 229 / 231
\item Cooperator Hunter: 223 / 241 / 253
\item SelfSteem: 224 / 230 / 234
\item SolutionB1: 225 / 243 / 258
\item Cycler CCD: 226 / 231 / 239
\item Meta Winner Long Memory: 134 players: 227 / 216 / 189
\item Meta Winner: 213 players: 228 / 217 / 192
\item Alternator: 229 / 236 / 241
\item k63r: 230 / 240 / 248 / 57
\item Meta Winner Deterministic: 146 players: 231 / 218 / 190
\item ZD-Extort-2 v2: 0.125, 0.5, 1: 232 / 214 / 196
\item ZD-Extort-2: 0.1111111111111111, 0.5: 233 / 213 / 197
\item Meta Winner Ensemble: 213 players: 234 / 232 / 208
\item Meta Winner Stochastic: 67 players: 235 / 233 / 209
\item Win-Shift Lose-Stay: D: 236 / 244 / 247
\item Meta Winner Finite Memory: 79 players: 237 / 225 / 201
\item Cycler DC: 238 / 242 / 246
\item Meta Winner Memory One: 36 players: 239 / 234 / 207
\item k50r: 240 / 235 / 249 / 54
\item TF1: 241 / 238 / 224
\item ThueMorse: 242 / 250 / 256
\item Cycler DDC: 243 / 257 / 257
\item ZD-Extort3: 0.11538461538461539, 0.3333333333333333, 1: 244 / 226 / 213
\item AntiCycler: 245 / 259 / 263
\item Predator: 246 / 247 / 235
\item k36r: 247 / 251 / 243 / 63
\item ZD-Extort-4: 0.23529411764705882, 0.25, 1: 248 / 239 / 221
\item ThueMorseInverse: 249 / 248 / 251
\item CollectiveStrategy: 250 / 246 / 227
\item $\pi$: 251 / 260 / 264
\item UsuallyDefects: 252 / 249 / 237
\item Tricky Cooperator: 253 / 256 / 260
\item ZD-Mischief: 0.1, 0.0, 1: 254 / 237 / 223
\item Aggravater: 255 / 254 / 233
\item Better and Better: 256 / 258 / 242
\item ZD-Extortion: 0.2, 0.1, 1: 257 / 245 / 232
\item $e$: 258 / 261 / 265
\item First by Anonymous: 259 / 253 / 254
\item krandomc: 260 / 252 / 255 / 62
\item Bush Mosteller: 0.5, 0.5, 3.0, 0.5: 261 / 255 / 250
\item Desperate: 262 / 263 / 262
\item Gradual Killer: (D, D, D, D, D, C, C): 263 / 266 / 267
\item Meta Minority: 213 players: 264 / 268 / 268
\item Hopeless: 265 / 265 / 266
\item Bully: 266 / 269 / 269
\item Defector: 267 / 262 / 240
\item Handshake: 268 / 264 / 252
\item Tricky Defector: 269 / 267 / 261
\item $\phi$: 270 / 270 / 271
\item Negation: 271 / 271 / 270
\item Anti Tit For Tat: 272 / 272 / 272
